# Supplementary material for: Quantum Memory Enhanced Multipoint Correlation Spectroscopy for Statistically Polarized NMR
Source: arXiv:2503.18930 source file (2025-12-17)
Supplement: Supplementary file 2 [file label_definitions_supp.tex]

\setcounter{figure}{0}
\setcounter{equation}{0}
\setcounter{section}{0}
